# Supplementary material for: Online Bayesian Persuasion Without a Clue
Source: arXiv:2411.06141 source file (2024-11-09)
Supplement: Supplementary file 2 [file appendix_h_representation.tex]

\section{On the computation complexity of Algorithm~\ref{alg:find_signaling_scheme}}\label{appendix:h_representation}

\bollo{Questa appendix si dovrebbe poter togliere}

Algorithm~\ref{alg:find_signaling_scheme} takes in input the set of vertices $\mathcal{V}$ and the corresponding best responses $(a(x))_{x \in \mathcal{V}}$.  
Then, it solves an LP with a number of variables equal to $|\mathcal{V}|$.
As the size of $\mathcal{V}$ can be exponential in $n$ and $d$, Algorithm~\ref{alg:find_signaling_scheme} requires exponential CPU time and memory space.
%\bollo{vorrei evitare confusione tra il numero di sample e la time complexity} 
In order to solve this problem, we rewrite the LP in terms of the H-representation of the polytopes $\mathcal{X}_\epsilon(a)$.
Furthermore, we provide a variation of Algorithm~\ref{alg:find_partition} that computes the H-representations efficiently.
This way, Algorithm~\ref{alg:main_algorithm} requires polynomial CPU time and memory space at each time step $t \in [T]$.

\subsection{Building the H-representation}

We observe that Algorithm~\ref{alg:find_partition} first finds the H-representation of every polytope $\mathcal{X}_\epsilon(a_i)$ such that $\text{vol}(\mathcal{X}_\epsilon(a_i)) > 0$, and places the action $a_i$ in the set $\mathcal{C}$.
However, to find the optimal signaling scheme, we have also to take into account the actions outside the set $\mathcal{C}$, which correspond to regions $\mathcal{X}_\epsilon(a_j)$ with $\text{vol}(\mathcal{X}_\epsilon(a_j)) = 0$.
%
%\bac{ quale issue? }The issue is due to the presence of polytopes $\mathcal{X}_\epsilon(a)$ with null volume.
%

At Line~\ref{line:query_vertices}, Algorithm~\ref{alg:find_partition} finds, for every %\bac{some? } \bollo{credo che sia giusto every}
polytope $\mathcal{X}_\epsilon(a_j)$ with $\text{vol}(\mathcal{X}_\epsilon(a_j))=0$, the vertices $x $ that belong to $ V(\mathcal{X}_\epsilon(a_j))$ where $a(x)=a_j$.
Since the number of these vertices can be exponential in the number of actions $n$ and in the number of states $d$, Algorithm~\ref{alg:find_partition} may return an exponentially large set.
Consequently, Algorithm~\ref{alg:find_signaling_scheme} in Phase~3 may instantiate an LP with exponentially many variables, which cannot be solved efficiently.
%
% Subsequently, by repeatably solving an LP that takes this set of vertices as input, Algorithm~\ref{alg:find_signaling_scheme} requires exponential CPU time and memory at every time step. 
%
%Here we show how to build, with the same number of samples \bac{qui specificherei meglio}, the H-representation of a (possibly improper) face of $\mathcal{X}_\epsilon(a)$ that contains all those vertices.

Here we show how to build, for every action $a_j \notin \mathcal{C}$, the H-representation of a (possibly improper) face of $\mathcal{X}_\epsilon(a_j)$ that contains all those vertices $x \in V(\mathcal{X}_\epsilon(a_j))$ where $a(x)=a_j$.
This procedure executes the same number of queries performed by Line~\ref{line:query_vertices} Algorithm~\ref{alg:find_partition}, and has polynomial time and space complexity at each time step.
Thus, it can be used in place of Line~\ref{line:query_vertices} to produce the H-representation of the regions $\mathcal{X}(a)$.
Then, during Phase~3, we can solve an LP that works directly on the H-representations to find an optimal signaling with polynomial time and space complexity at each time step.

For every $a_i \in \mathcal{C}$, we will denote with $\mathcal{R}^\text{H}(\mathcal{X}_\epsilon(a_i))$ the set of hyperplanes corresponding to the minimal H-representation of $\mathcal{X}_\epsilon(a_i)$.
This set includes every separating hyperplane $H_{ik}$ found by Algorithm~\ref{alg:find_partition}, together with the non-redundant boundary hyperplanes that delimit $\mathcal{X}_\epsilon$. 

Furthermore, we let $\mathcal{V}$ be the set of all vertices of the regions $\mathcal{X}^{\triangle}_\epsilon(a)$, formally:
\begin{equation*}
	\mathcal{V} \coloneqq \bigcup_{a \in \mathcal{A}} V(\mathcal{X}^{\triangle}_\epsilon(a)).
\end{equation*}
As we will prove later (see Lemma~\ref{lem:zero_vol_face}), this set is equivalent to $\bigcup_{a \in \mathcal{C}} V(\mathcal{X}^{\triangle}_\epsilon(a))$, which is the set taken in input by Algorithm~\ref{alg:find_signaling_scheme}.
%Such a set is a parameter of Program~\ref{eq:lp_two_signals}.
With an abuse of notation, we define the set of vertices where an action $a \in \mathcal{A}$ is a best-response as:
\begin{equation*}
	\mathcal{V}(a) \coloneqq \{x \in V(\mathcal{X}^{\triangle}_\epsilon(a)) \mid a(x)=a\}.
\end{equation*}

Suppose, for the sake of presentation, that there exists a single polytope $\mathcal{X}_\epsilon(a_j)$ with zero volume.
Then, given the H-representation of the other polytopes $\mathcal{X}_\epsilon(a_i)$, Algorithm~\ref{alg:zero_vol_h_representation} reaches our goal.
Such an algorithm can be easily extended to the case with multiple polytopes with zero volume in order to substitute Line~\ref{line:query_vertices} Algorithm~\ref{alg:find_partition}. \bac{ricordarsi poi di sostituirla effetivamnte}

Algorithm~\ref{alg:zero_vol_h_representation} iterates over the vertices of the regions with volume larger than zero, which include all the vertices of the region $\mathcal{X}_\epsilon(a_j)$.
While doing so, it builds a set of hyperplanes $\mathcal{H}(a_i) \subseteq \mathcal{R}^\text{H}(\mathcal{X}_\epsilon(a_i))$ for every action $a_i \in \mathcal{C}$.
Such a (possibly empty) set includes all and only the hyperplanes in $\mathcal{R}^\text{H}(\mathcal{X}_\epsilon(a_i))$ that contain all the vertices where the action $a_j$ has been observed, \emph{i.e}, $a(x)=a_j$.
Finally, at Line~\ref{line:return_h_representation} Algorithm~\ref{alg:zero_vol_h_representation} intersects every region $\mathcal{X}_\epsilon(a_i)$ with the corresponding hyperplanes in $\mathcal{H}(a_i)$.
Finally, as we show in the following, this intersection is always non-empty and corresponds to the output of Algorithm~\ref{alg:zero_vol_h_representation}.
%We can prove that at least one intersection is non-empty.
%This intersection is returned by the algorithm.
 
%\begin{wrapfigure}[14]{R}{0.5\textwidth}
%	\vspace{-0.85cm}
%	\begin{minipage}{0.5\textwidth}
\begin{algorithm}[H]
	\caption{\texttt{Find-H-Representation}}%\label{alg:zero_vol_h_representation}
	\begin{algorithmic}[1]
		\Require $\mathcal{X}_\epsilon(a_i), \mathcal{R}^\text{H}(\mathcal{X}_\epsilon(a_i)) \quad \forall a_i \in \mathcal{C}$ 
		\State $\mathcal{H}(a_i) \gets \emptyset \quad \forall a_i \in \mathcal{C}$ 
%		\State $x \gets $ the first vertex of $\mathcal{X}_\epsilon(a_j)$
%		\State \bollo{linea sopra andrebbe riscritta meglio}
%		\State $\mathcal{H}(a_i) \gets \{H \in \mathcal{R}^\text{H}(\mathcal{X}_\epsilon(a_i)) \mid x \in H \} \quad \forall a_i \in \mathcal{C}$% : x \in V(\mathcal{X}_\epsilon(a_i))$
		\State $\texttt{First} \gets \texttt{True}$
		\ForAll{$x \in \bigcup_{a_i \in \mathcal{C}}V(\mathcal{X}_\epsilon(a_i))$}
		\State $a \gets \texttt{Action-Oracle}(x)$
		\If{$a = a_j$}
		\If{$\texttt{First} = \texttt{False}$}
		\State $\mathcal{H}(a_i) \gets \{H \in \mathcal{R}^\text{H}(\mathcal{X}_\epsilon(a_i)) \mid x \in H, H \in \mathcal{H}(a_i) \} \quad \forall a_i \in \mathcal{C}$% : x \in V(\mathcal{X}_\epsilon(a_i))$
%		\State $\mathcal{H}(a_i) \gets \emptyset \quad \forall a_i \in \mathcal{C} : x \notin V(\mathcal{X}_\epsilon(a_i))$
		\Else
		\State $\mathcal{H}(a_i) \gets \{H \in \mathcal{R}^\text{H}(\mathcal{X}_\epsilon(a_i)) \mid x \in H \} \quad \forall a_i \in \mathcal{C}$% : x \in V(\mathcal{X}_\epsilon(a_i))$
		\State $\texttt{First} \gets \texttt{False}$
		\EndIf
		\EndIf
		\EndFor
		\State \textbf{Return} $\mathcal{X}_\epsilon(a_i) \cap \bigcap_{H \in \mathcal{H}(a_i)}H$ for any $a_i$ such that $\mathcal{X}_\epsilon(a_i) \cap \bigcap_{H \in \mathcal{H}(a_i)}H \neq \emptyset$ %\label{line:return_h_representation}
	\end{algorithmic}
\end{algorithm}
%	\end{minipage}
%\end{wrapfigure}

\bac{Metterei un lemma iniziale su quello che fa l'algoritmo 12, del tipo: L'algoritmo 12 calcola una faccia ... con $O(\binom{m+d}{d})$. Aiuta molto se uno vuole saltare due pagine di lemmi tecnici.}

The main result concerning Algorithm~\ref{alg:zero_vol_h_representation} is the following:
\begin{restatable}{lemma}{FindHReprZeroVol}
	If there is a single polytope $\mathcal{X}_\epsilon(a_j)$ such that $\text{vol}(\mathcal{X}_\epsilon(a_j))=0$, then Algorithm~\ref{alg:zero_vol_h_representation} returns a (possibly improper) face $\mathcal{F}(a_j)$ of $\mathcal{X}_\epsilon(a_j)$ such that, every vertex $x \in V(\mathcal{X}_\epsilon(a_j))$, if $a(x)=a_j$, then $x \in \mathcal{F}(a_j)$.
	Furthermore, the Algorithm requires $|\bigcup_{a_i \in \mathcal{C}} V(\mathcal{X}(a_i))|$ calls to Algorithm~\ref{alg:action_oracle}, and has polynomial time and space complexity between each two consecutive queries.
\end{restatable}

In order to prove it, we first need to introduce two technical lemmas to characterize the relationship between regions with null volume and those with volume larger than zero.

\begin{restatable}{lemma}{zeroVolFace2}
	%\label{lem:intersection_zero_vol_face}
	Let $a_i, a_j \in \mathcal{A}$ such that $\text{vol}(\mathcal{X}_\epsilon(a_i))>0$ and $\text{vol}(\mathcal{X}_\epsilon(a_j))=0$.
	Then $\mathcal{X}_\epsilon(a_i) \cap \mathcal{X}_\epsilon(a_j)$ is a (possibly improper) face of $\mathcal{X}_\epsilon(a_i)$ and $\mathcal{X}_\epsilon(a_j)$.
\end{restatable}
\begin{proof}
	In the following we assume that $\mathcal{X}_\epsilon(a_i) \cap \mathcal{X}_\epsilon(a_j)$ is non-empty, as the empty set is an improper face of every polytope.
	
	\bac{in generale se devi provare l'uguaglianza tra due set $A,B$ il modo piu chiaro secondo me e $A \subseteq B$ e $B \subseteq A$}
	
	We prove that $\mathcal{X}_\epsilon(a_i) \cap \mathcal{X}_\epsilon(a_j) = \mathcal{X}_\epsilon(a_i) \cap H_{ij} = \mathcal{X}_\epsilon(a_j) \cap H_{ij}$.
	In order to do that, we first show that $\mathcal{X}_\epsilon(a_i) \cap H_{ij} \subseteq \mathcal{X}_\epsilon(a_i) \cap \mathcal{X}_\epsilon(a_j)$.
	Consider a normalized slice $x \in \mathcal{X}_\epsilon(a_i) \cap H_{ij}$.
	Then we have that$x \in \mathcal{X}_\epsilon(a_j)$.
	As this holds for every $x \in \mathcal{X}_\epsilon(a_i) \cap H_{ij}$, it follows that $\mathcal{X}_\epsilon(a_i) \cap H_{ij} \subseteq \mathcal{X}_\epsilon(a_i) \cap \mathcal{X}_\epsilon(a_j)$.
	
	Similarly, we show that $\mathcal{X}_\epsilon(a_i) \cap \mathcal{X}_\epsilon(a_j) \subseteq \mathcal{X}_\epsilon(a_i) \cap H_{ij}$.
	Take any normalized slice $x \in \mathcal{X}_\epsilon(a_i) \cap \mathcal{X}_\epsilon(a_j)$. 
	Then $x \in H_{ij}$ as it belongs to both $\mathcal{X}_\epsilon(a_i)$ and $\mathcal{X}_\epsilon(a_j)$, thus $x \in \mathcal{X}_\epsilon(a_i) \cap H_{ij}$.
	This implies that $\mathcal{X}_\epsilon(a_i) \cap \mathcal{X}_\epsilon(a_j) \subseteq \mathcal{X}_\epsilon(a_i) \cap H_{ij}$.
	
	Consequently, we have that $\mathcal{X}_\epsilon(a_i) \cap \mathcal{X}_\epsilon(a_j) = \mathcal{X}_\epsilon(a_i) \cap H_{ij}$.
	With a similar argument, we can prove that $\mathcal{X}_\epsilon(a_i) \cap \mathcal{X}_\epsilon(a_j) = \mathcal{X}_\epsilon(a_j) \cap H_{ij}$.
	As a result, we have that $\mathcal{X}_\epsilon(a_i) \cap \mathcal{X}_\epsilon(a_j) = \mathcal{X}_\epsilon(a_i) \cap H_{ij} = \mathcal{X}_\epsilon(a_j) \cap H_{ij}$.
	
	In order to conclude the proof, we show that $\mathcal{X}_\epsilon(a_i) \cap \mathcal{X}_\epsilon(a_j) = \mathcal{X}_\epsilon(a_i) \cap H_{ij} = \mathcal{X}_\epsilon(a_j) \cap H_{ij}$ is a face of both $\mathcal{X}_\epsilon(a_i)$ and $\mathcal{X}_\epsilon(a_j)$.
	We observe that $\mathcal{X}_\epsilon(a_i) \subseteq \mathcal{H}_{ij}$,\bac{non capisco il senso di questa inclusione} thus the non-empty region $\mathcal{X}_\epsilon(a_i) \cap H_{ij}$ is by definition a face of $\mathcal{X}_\epsilon(a_i)$.
	Similarly, $\mathcal{X}_\epsilon(a_j) \subseteq \mathcal{H}_{ji}$, thus the non-empty region $\mathcal{X}_\epsilon(a_j) \cap H_{ij}$ is a face of $\mathcal{X}_\epsilon(a_j)$ (possibly the improper face $\mathcal{X}_\epsilon(a_j)$ itself).
\end{proof}

\begin{restatable}{lemma}{zeroVolFace}
	%\label{lem:zero_vol_face}
	Let $\mathcal{X}_\epsilon(a_j)$ be a polytope such that $\text{vol}(\mathcal{X}_\epsilon(a_j))=0$.
	Then $\mathcal{X}_\epsilon(a_j)$ is a face of some polytope $\mathcal{X}_\epsilon(a_i)$ with $\text{vol}(\mathcal{X}_\epsilon(a_i))>0$.
\end{restatable}
\begin{proof}
	
	First, we observe that if $\mathcal{X}_\epsilon(a_j)$ is empty, then it is the improper face of any region $\mathcal{X}_\epsilon(a_i)$ with $\text{vol}(\mathcal{X}_\epsilon(a_i))>0$.
	Thus, in the following, we consider $\mathcal{X}_\epsilon(a_j)$ to be non-empty.
	
	As a first step, we observe that any normalized slice $x \in \mathcal{X}_\epsilon(a_j)$ belongs also to some region $\mathcal{X}_\epsilon(a_k)$, where $a_k \in \mathcal{A}$ depends on $x$, such that $\text{vol}(\mathcal{X}_\epsilon(a_k))>0$.
	Suppose, by contradiction, that $x \in \text{int}(\mathcal{X}_\epsilon(a_i))$.
	Then $a_i$ is a best-response in $\mathcal{X}_\epsilon(a_j) \cap \mathcal{H}_{ij}$, \emph{i.e.}, $\mathcal{X}_\epsilon(a_j) \cap \mathcal{H}_{ij} \subseteq \mathcal{X}_\epsilon(a_i)$.
	One can easily observe that such a region has positive volume, thus contradicting the hypothesis that $\text{vol}(\mathcal{X}_\epsilon(a_j))=0$.
	
	Now we prove that there exists some $\mathcal{X}_\epsilon(a_i)$ with $\text{vol}(\mathcal{X}_\epsilon(a_i))>0$ such that $\mathcal{X}_\epsilon(a_j) \subseteq \mathcal{X}_\epsilon(a_i)$. 
	If $\mathcal{X}_\epsilon(a_j)$ is a single normalized slice $x$, then this trivially holds.
	
	Suppose instead that $\mathcal{X}_\epsilon(a_j)$ has dimension at least one.
	Consider a fixed normalized slice $\bar{x} \in \text{int}(\mathcal{X}_\epsilon(a_j))$, where the interior is taken relative to the subspace that contains $\mathcal{X}_\epsilon(a_j)$ and has minimum dimension.
	There exists a region $\mathcal{X}_\epsilon(a_i)$ with $\text{vol}(\mathcal{X}_\epsilon(a_i))>0$ such that $\bar{x} \in \mathcal{X}_\epsilon(a_i)$.
	
	We prove that $\mathcal{X}_\epsilon(a_j) \subseteq \mathcal{X}(a_i)$.
	Suppose, by contradiction, that there exists a normalized slice $x \in \mathcal{X}_\epsilon(a_j)$ such that $x \notin \mathcal{X}_\epsilon(a_i)$.
	It follows that the line segment $\text{co}(\bar{x},x)$ intersect the separating hyperplane $H_{ij}$ in some normalized slice $\widetilde{x} \in \text{co}(\bar{x},x) \cap H_{ij}$.
	Furthermore, since $\widetilde{x} \neq x$ and $\bar{x} \in \text{int}(\mathcal{X}_\epsilon(a_j))$, then $\widetilde{x} \in \text{int}(\mathcal{X}_\epsilon(a_j))$.
	However, if the internal point $\widetilde{x}$ belongs to the hyperplane $H_{ij}$ and $\mathcal{X}_\epsilon(a_j) \subseteq \mathcal{H}_{ji}$, then it must be the case that $\mathcal{X}_\epsilon(a_j) \subseteq H_{ij}$.
	This implies that $\mathcal{X}_\epsilon(a_j) \subseteq \mathcal{X}_\epsilon(a_i)$ and thus $x \in \mathcal{X}_\epsilon(a_i)$, which contradicts the hypothesis.. 
	
	Given that there exists some $\mathcal{X}_\epsilon(a_i)$ with $\text{vol}(\mathcal{X}_\epsilon(a_i))>0$ such that $\mathcal{X}_\epsilon(a_j) \subseteq \mathcal{X}_\epsilon(a_i)$, then $\mathcal{X}_\epsilon(a_j) = \mathcal{X}_\epsilon(a_i) \cap \mathcal{X}_\epsilon(a_j)$ is a face of $\mathcal{X}_\epsilon(a_i)$ by Lemma~\ref{lem:intersection_zero_vol_face}.
\end{proof}
%\bollo{Corollary: ogni facca di $X(a_j)$ è una faccia di una regione a volume non nullo}

\FindHReprZeroVol
\begin{proof}
	In the following, for the sake of notation, given a polytope $\mathcal{X}_\epsilon(a)$ and the a set of hyperplanes $\mathcal{H}(a)$, with an abuse of notation we denote with $\mathcal{X}_\epsilon(a) \cap \mathcal{H}(a)$ the intersection of $\mathcal{X}_\epsilon(a)$ with every hyperplane in $\mathcal{H}(a)$.
	Formally:
	\begin{equation}
		%\label{eq:abuse_intersect_x_h}
		\mathcal{X}_\epsilon(a) \cap\ \mathcal{H}(a) \coloneqq \mathcal{X}_\epsilon(a) \cap \bigcap_{H \in \mathcal{H}(a)} H.
	\end{equation}
		
	Let $a_i$ be action selected at Line~\ref{line:return_h_representation} Algorithm~\ref{alg:zero_vol_h_representation}.
	We denote with $\mathcal{F}(a_i)$ the face returned by Algorithm~\ref{alg:zero_vol_h_representation}:
	\begin{equation*}
		\mathcal{F}(a_i) \coloneqq \mathcal{X}_\epsilon(a_i) \cap \mathcal{H}(a_i).
	\end{equation*}
%	Furthermore, we denote with $\mathcal{W}$ the set of vertices where action $a_j$ is observed:
%	\begin{equation*}
%		\mathcal{W} \coloneqq \{x \in V(\mathcal{X}_\epsilon(a_j)) \mid a(x) = a_j\}.
%	\end{equation*}
	We observe that by Lemma~\ref{lem:zero_vol_face}, there exists some action $a_k \in \mathcal{C}$ such that $\mathcal{X}_\epsilon(a_j)$ is a face of $\mathcal{X}_\epsilon(a_k)$.
	Consequently, Algorithm~\ref{alg:zero_vol_h_representation} queries every vertex $x \in \mathcal{V}(a_j)$.	
	
	As a first step we show that $\mathcal{F}(a_i)$ actually is a face of $\mathcal{X}_\epsilon(a_i)$ and contains every vertex of $\mathcal{V}(a_j)$.
	Being the non-empty intersection of $\mathcal{X}_\epsilon(a_i)$ with some hyperplanes in $\mathcal{R}^\text{H}(\mathcal{X}_\epsilon(a_i))$, $\mathcal{F}(a_i)$ is a face of $\mathcal{X}_\epsilon(a_i)$.
	One can easily prove by induction that $\mathcal{H}(a_i)$ includes all and only the hyperplanes within $\mathcal{R}^\text{H}(\mathcal{X}_\epsilon(a_i))$ containing every vertex in $\mathcal{V}(a_j)$.
	Thus, $\mathcal{V}(a_j) \subseteq \mathcal{F}(a_i)$.
	
%	Furthermore, there exists an action $a_i$ that Algorithm~\ref{alg:zero_vol_h_representation} can selects at Line~\ref{line:return_h_representation}, \emph{i.e.}, such that $\mathcal{F}(a_i)$ is non-empty.
%	Thanks to Lemma~\ref{lem:zero_vol_face}, there exists some action $a_k \in \mathcal{C}$ such that $\mathcal{X}_\epsilon(a_j)$ is a face of $\mathcal{X}_\epsilon(a_k)$.
%	Consequently the algorithm can always select $a_i = a_j$. 
	
	Now we show that $\mathcal{F}(a_i)$ is not only a (proper) face of $\mathcal{X}_\epsilon(a_i)$ containing the set $\mathcal{V}(a_j)$, but also a face of $\mathcal{X}_\epsilon(a_j)$ (possibly the improper face $\mathcal{X}_\epsilon(a_j)$ itself).
	We consider the set $\mathcal{X}_\epsilon(a_i) \cap \mathcal{X}_\epsilon(a_j)$, which is a face of both $\mathcal{X}_\epsilon(a_i)$ and $\mathcal{X}_\epsilon(a_j)$ as for Lemma~\ref{lem:intersection_zero_vol_face}.
	Thus, there exists some set of hyperplanes $\mathcal{H}'(a_i) \subset \mathcal{R}^\text{H}(\mathcal{X}_\epsilon(a_i))$ such that:
	\begin{equation}
		%\label{eq:h_repr_i_cap_j}
		\mathcal{X}_\epsilon(a_i) \cap \mathcal{H}'(a_i) = \mathcal{X}_\epsilon(a_i) \cap \mathcal{X}_\epsilon(a_j).
	\end{equation}
	Furthermore, we observe that $\mathcal{V}(a_j) \subseteq \mathcal{X}_\epsilon(a_i) \cap \mathcal{X}_\epsilon(a_j)$.
	Indeed, we have that $\mathcal{V}(a_j) \subseteq \mathcal{X}_\epsilon(a_i)$ since $\mathcal{V}(a_j) \subseteq \mathcal{F}(a_i)$ and $\mathcal{F}(a_i)$ is a face of $\mathcal{X}_\epsilon(a_i)$, and $\mathcal{V}(a_j) \subseteq \mathcal{X}_\epsilon(a_j)$ by definition.
	
	We want to prove that $\mathcal{H}'(a_i) \subseteq \mathcal{H}(a_i)$, where the set $\mathcal{H}(a_i)$ contains all and only the hyperplanes within $\mathcal{R}^\text{H}(\mathcal{X}_\epsilon(a_i))$ that include the whole set $\mathcal{V}(a_j)$.
	In order to do that, suppose, by contradiction, that there exists a vertex $x \in \mathcal{V}(a_j)$ such that $x \notin H$ for some $H \in \mathcal{H}'(a_i)$.
	Then, $x \notin \mathcal{X}_\epsilon(a_i) \cap \mathcal{H}'(a_i) \subseteq H$.
	However, we proved that $\mathcal{V}(a_j) \subseteq \mathcal{X}_\epsilon(a_i) \cap \mathcal{X}_\epsilon(a_j)$ and $\mathcal{X}_\epsilon(a_i) \cap \mathcal{X}_\epsilon(a_j) = \mathcal{X}_\epsilon(a_i) \cap \mathcal{H}'(a_i)$ by definition of $\mathcal{H}'(a_i)$, reaching a contradiction.
	
	Consequently:
	\begin{align*}
		\mathcal{F}(a_i) \coloneqq 	\mathcal{X}_\epsilon(a_i) \cap \mathcal{H}(a_i) &= \mathcal{X}_\epsilon(a_i) \cap \bigcap_{H \in \mathcal{H}(a_i)} H \\
		&\subseteq \mathcal{X}_\epsilon(a_i) \cap \bigcap_{H \in \mathcal{H}'(a_i)} H \\
		&= \mathcal{X}_\epsilon(a_i) \cap \mathcal{H}'(a_i) \\
		&= \mathcal{X}_\epsilon(a_i) \cap \mathcal{X}_\epsilon(a_j),
	\end{align*}
	where we applied Equation~\ref{eq:abuse_intersect_x_h}, the fact that $\mathcal{H}'(a_i) \subseteq \mathcal{H}'(a_j)$, and Equation~\ref{eq:h_repr_i_cap_j}.
	
	Finally, we can show that $\mathcal{F}(a_i)$ is a face of $\mathcal{X}_\epsilon(a_j)$.
	We have that $\mathcal{F}(a_i)$ is a face of $\mathcal{X}_\epsilon(a_i)$ and $\mathcal{F}(a_i) \subseteq \mathcal{X}_\epsilon(a_i) \cap \mathcal{X}_\epsilon(a_j)$, which is itself a face of $\mathcal{X}_\epsilon(a_i)$ by Lemma~\ref{lem:intersection_zero_vol_face}.
	Thus, $\mathcal{F}(a_i)$ is a face of $\mathcal{X}_\epsilon(a_i) \cap \mathcal{X}_\epsilon(a_j)$.
	Furthermore, Lemma~\ref{lem:intersection_zero_vol_face} states that $\mathcal{X}_\epsilon(a_i) \cap \mathcal{X}_\epsilon(a_j)$ is also a face of $\mathcal{X}_\epsilon(a_j)$.
	This implies that $\mathcal{F}(a_i)$ is a face of a face of $\mathcal{X}_\epsilon(a_j)$, and thus a face of $\mathcal{X}_\epsilon(a_j)$ itself. 
	
	In order to conclude the proof, we have to prove that at Line~\ref{line:return_h_representation} Algorithm~\ref{alg:zero_vol_h_representation} can actually find an action $a_i$ such that $\mathcal{F}(a_i) = \mathcal{X}_\epsilon(a_i) \cap \mathcal{H}(a_i)$ is non-empty.
	Let $a_k \in \mathcal{C}$ be such that $\mathcal{X}_\epsilon(a_j)$ is a face of $\mathcal{X}_\epsilon(a_k)$, which exists thanks to Lemma~\ref{lem:zero_vol_face}.
	Let $x$ be any vertex in the set $\mathcal{V}(a_j)$ and define $\mathcal{H}''(a_j)$ as:
	\begin{equation*}
		\mathcal{H}''(a_k) \coloneqq \{H \in \mathcal{R}^H(\mathcal{X}_\epsilon(a_k)) \mid x \in H \}.
	\end{equation*}
	Then $\mathcal{X}_\epsilon(a_k) \cap \mathcal{H}''(a_k) = \{x\}$.
	Consequently, $\mathcal{H}(a_k) \subseteq \mathcal{H}''(a_k)$, and thus:
	\begin{align*}
		\mathcal{X}_\epsilon(a_k) \cap \mathcal{H}(a_k) &= \mathcal{X}_\epsilon(a_k) \cap \bigcap_{H \in \mathcal{H}(a_k)} H \\
		&\subseteq \mathcal{X}_\epsilon(a_k) \cap \bigcap_{H \in \mathcal{H}''(a_k)} H \\
		&= \mathcal{X}_\epsilon(a_k) \cap \mathcal{H}''(a_k) \\
		&= \{x\} \neq \emptyset.
	\end{align*}
	As a result, there is always an action $a_k \in \mathcal{C}$ such that $\mathcal{X}_\epsilon(a_k) \cap \mathcal{H}(a_k) \neq \emptyset$.
	
	Finally, we observe that Algorithm~\ref{alg:zero_vol_h_representation} executes Algorithm~\ref{alg:action_oracle} once for every vertex in the set $\bigcup_{a_i \in \mathcal{C}} V(\mathcal{X}_\epsilon(a_i))$, and the operations it performs between two consecutive queries have polynomial time and space complexity.
\end{proof}

\subsection{Finding the signaling scheme}
Thanks to Algorithm~\ref{alg:find_partition} and Algorithm~\ref{alg:zero_vol_h_representation}, we can build the H-representation of the ``important'' part of every region $\mathcal{X}_\epsilon(a_i)$.
Formally, for every action $a \in \mathcal{A}$, under the events $\mathcal{E}_1$ and $\mathcal{E}_2$ we acquire the H-representation of some region $\mathcal{R}_\epsilon^{\triangle}(a)$.
In particular, for every action $a_i \in \mathcal{C}$, we have that $\mathcal{R}_\epsilon^{\triangle}(a_i) = \mathcal{X}_\epsilon(a_i)$.
On the other hand, for every action $a_j \notin \mathcal{C}$, we have that $\mathcal{R}_\epsilon^{\triangle}(a_j)$ is either $\mathcal{X}_\epsilon(a_j)$ or a face of $\mathcal{X}_\epsilon(a_j)$ such that $\mathcal{V}(a_j) \subseteq \mathcal{R}^{\triangle}_\epsilon(a_j)$.
% such that $\mathcal{F}^{\triangle}(a)$ is a (possibly improper) face of $\mathcal{X}_\epsilon^{\triangle}(a)$ containing every vertex $x \in V(\mathcal{X}_\epsilon^{\triangle}(a))$ where $a(x)=a$.
Furthermore, we can build the regions $\mathcal{R}_\epsilon^{\Hsquare}(a)$ by keeping the separating half-spaces and intersecting them with the space of slices $\mathcal{X}_\epsilon^{\Hsquare}$ instead of the space of normalized slices $\mathcal{X}_\epsilon^{\triangle}$.

Given these region, we provide Algorithm~\ref{alg:find_sig_scheme_h_repr} to find an approximately optimal signaling scheme.
\begin{algorithm}[H]
	\caption{\texttt{Compute-Signaling-H-Representation}}%\label{alg:find_sig_scheme_h_repr}
	\begin{algorithmic}[1]
		\Require $\mathcal{R}^{\Hsquare}_\epsilon(a) \quad \forall a \in \mathcal{A}$, $\X_\epsilon$, $\widehat{\mu}_t \in \Delta_{\Theta}$
		\State Solve Program~\eqref{eq:lp_h_repr} for an optimal solution $\psi = \varphi^\star$:
		%\vspace{-4mm}
		\begin{align}
			\max_{\psi \ge 0} & \,\, \sum_{a \in \mathcal{A}}  \sum_{\theta \in \Theta}  \widehat{\mu}_{t,\theta} \varphi^a_\theta u^\text{s}_\theta(a) \quad \text{s.t.} %\label{eq:lp_h_repr}\\
			& \varphi^a \in \mathcal{R}^{\Hsquare}_\epsilon(a) \quad \forall a \in \mathcal{A} \nonumber \\
			& \sum_{a \in \mathcal{A}} \varphi^a_\theta \le 1 \quad \forall \theta \in \Theta \nonumber
		\end{align}
		%\vspace{-2mm}
		%\end{subequations}
		\State $\sset \gets \{ s^\star \} \cup \left\{ s^a \mid a \in \mathcal{A} \right\}$
		\For{$\theta \in \Theta$}
		\State $
		\phi_\theta \hspace{-.5mm} \gets \hspace{-.5mm} \begin{cases}
			\phi_{\theta}(s^{a}) = \psi^a_\theta \,\,\,\, \forall a \in \mathcal{A} \\
			\phi_{\theta}(s^{\star}) = 1 - \sum_{a \in \mathcal{A} }\psi^a_\theta
		\end{cases}
		$
		\EndFor
		\State\Return $\phi$
	\end{algorithmic}
\end{algorithm}

We observe that given the H-representation of the regions $\mathcal{R}^{\Hsquare}_\epsilon(a)$, which includes $\mathcal{O}(n+d)$ hyperplanes, Program~\ref{eq:lp_h_repr} can be solved in polynomial time.

\begin{restatable}{lemma}{HReprFindSignal}
	Let Algorithm~\ref{alg:find_sig_scheme_h_repr} have in input, for every action $a \in \mathcal{A}$, a face $\mathcal{R}^{\Hsquare}(a)$ of $\mathcal{X}_\epsilon^{\Hsquare}(a)$ (possibly the improper face $\mathcal{X}^{\Hsquare}(a)$ itself) such that every vertex $x \in V(\mathcal{X}_\epsilon^{\Hsquare}(a))$ such that $a(x)=a$ belongs to $\mathcal{R}^{\Hsquare}_\epsilon(a)$.
	Then the signaling scheme $\phi$ output by the algorithm is $\mathcal{O}(  \epsilon n d  + \nu)$-optimal for $\nu \leq \left| \sum_{\theta \in \Theta} \widehat{\mu}_{t,\theta} - \mu_\theta \right|$	
%	Given inputs $\mathcal{Y}\coloneqq (\mathcal{V},[a(x)]_{x \in \mathcal{V}})$, $\X_\epsilon$, and $\widehat{\mu}_t \in \Delta_{\Theta}$ for Algorithm~\ref{alg:find_partition}, under events $\mathcal{E}_1$ and  $\mathcal{E}_2$, the signaling scheme $\phi$ output by the algorithm is $\mathcal{O}(  \epsilon n d  + \nu)$-optimal for $\nu \leq \left| \sum_{\theta \in \Theta} \widehat{\mu}_{t,\theta} - \mu_\theta \right|$
\end{restatable}
\begin{proof}
%	In the following we let $\mathcal{V}$ be the set of all vertices of the regions $\mathcal{X}^{\triangle}_\epsilon(a)$, formally:
%	\begin{equation*}
%		\mathcal{V} \coloneqq \bigcup_{a \in \mathcal{A}} V(\mathcal{X}^{\triangle}_\epsilon(a)).
%	\end{equation*}
%	Such a set is a parameter of Program~\ref{eq:lp_two_signals}.
%	With an abuse of notation, we define the set of vertices where an action $a \in \mathcal{A}$ is a best-response as:
%	\begin{equation*}
%		\mathcal{V}(a) \coloneqq \{x \in \mathcal{V} \mid a(x)=a\}.
%	\end{equation*}
	
	As a first step, we prove that given a feasible solution $\alpha$ for Program~\ref{eq:lp_two_signals}, one can construct a feasible solution $\varphi$ for Program~\ref{eq:lp_h_repr} with the same value.
	In particular, we consider a solution $\varphi$ defined as:
	\begin{equation*}
		\varphi^a_\theta \coloneqq \sum_{x \in \mathcal{V}(a)} \alpha_x x_\theta \quad \forall a \in \mathcal{A}, \theta \in \Theta.
	\end{equation*}
	
	We observe that for every $a \in \mathcal{A}$ and $\theta \in \Theta$ we can bound $\varphi^a_\theta$ as follows:
	\begin{align*}
		0 \le \varphi^A_\theta = \sum_{x \in \mathcal{V}(a)} \alpha_x x_\theta \le \sum_{x \in \mathcal{V}} \alpha_x x_\theta \le 1.
	\end{align*}
	Consequently, the vectors $\varphi^a$ belong to $\mathcal{X}^{\Hsquare}$.
	
	Let us define, for every $a \in \mathcal{A}$ and $x \in \mathcal{V}$, the coefficient:
	\begin{equation*}
		\beta^a_x \coloneqq \frac{\alpha_x}{\sum_{x \in \mathcal{V}(a)} \alpha_x}.
	\end{equation*}
	One can easily verify that $\beta^a \in \Delta_{\mathcal{V}(a)}$.
	Consider the normalized slice:
	\begin{equation*}
		x^a \coloneqq \sum_{x \in \mathcal{V}(a)} \beta^a_x x.
	\end{equation*}
	This slice belongs to $\mathcal{R}^{\triangle}_\epsilon(a)$, as it is the weighted sum of the vertices $\mathcal{V}(A) \subseteq V(\mathcal{R}^{\triangle}_\epsilon(a))$ with weights $\beta^a \in \Delta_{\mathcal{V}(a)}$.
	Furthermore, we can rewrite the solution $\varphi^a$ as:
	\begin{equation*}
		\varphi^a = x^a \sum_{x \in \mathcal{V}(a)} \alpha_x.
	\end{equation*} 
	Thus, by considering that $x^a \in \mathcal{R}^{\triangle}_\epsilon(a)$ and $\varphi^a \in \mathcal{X}^{\Hsquare}$, we have that $\varphi^a \in \mathcal{R}^{\Hsquare}_\epsilon(a)$.
	
	Finally, since $\alpha$ is a feasible solution for Program~\ref{eq:lp_two_signals}, we can observe that:
	\begin{equation*}
		\sum_{a \in \mathcal{A}} \varphi^a_\theta = \sum_{a \in \mathcal{A}} \sum_{x \in \mathcal{V}(a)} \alpha_x x = \sum_{x \in \mathcal{V}} \alpha_x x \le 1.
	\end{equation*}
	As a result, $\varphi$ is a feasible solution for Program~\ref{eq:lp_h_repr}.
	Direct calculations show that it achieves the same value of solution $\alpha$ for Program~\ref{eq:lp_two_signals}.
	It follows that the optimal solution of Program~\ref{eq:lp_h_repr} at least the value of the optimal solution of Program~\ref{eq:lp_two_signals}.
	
	As a further step we provide a lower bound on the utility of the signaling scheme computed by Algorithm~\ref{alg:find_sig_scheme_h_repr}.
%	In the following, we let $\psi$ be the optimal solution of Program~\ref{eq:lp_h_repr}.
	Let $\phi^{\textnormal{LP}}$ be the signaling scheme computed by Algorithm~\ref{alg:find_sig_scheme_h_repr}, while let $\Psi$ be the optimal solution to Program~\ref{eq:lp_h_repr}.
	Furthermore, we let $\psi$ be the optimal solution of Program~\ref{eq:lp_h_repr} and $\phi'$ the signaling scheme computed by Algorithm~\ref{alg:find_sig_scheme_h_repr} when $\widehat{\mu}:= \widehat \mu_t = \mu$.
	
	Since $\Psi^a \in \mathcal{R}^{\Hsquare}_\epsilon(a)$ for every $a \in \mathcal{A}$, we have that $a \in \mathcal{A}^{\phi^{\textnormal{LP}}}(a)$.
	Breaking ties in favor of the sender, the action $a^{\phi^{\textnormal{LP}}}(s^a)$ is such that:
	\begin{equation*}
		\sum_{\theta \in \Theta}  \mu_\theta \Psi^a_{\theta} u^\textnormal{s}_\theta (a^{\phi^{\textnormal{LP}}}(s^a)) \ge \sum_{\theta  \in \Theta}  \mu_\theta \Psi^a_{\theta} u^\textnormal{s}_\theta (a).
	\end{equation*}
	Then: 
	\begin{align*}
		u (\phi^{\textnormal{LP}}) & =  \sum_{s \in \mathcal{S} }  \sum_{\theta  \in \Theta}  \mu_\theta \phi^{\textnormal{LP}}_{\theta}(s) u^\textnormal{s}_\theta (a^{\phi^{\textnormal{LP}}}(s)) \\
		&\ge \sum_{s \in \mathcal{S} \setminus \{s^\star\} }  \sum_{\theta  \in \Theta}  \mu_\theta \phi^{\textnormal{LP}}_{\theta}(s) u^\textnormal{s}_\theta (a^{\phi^{\textnormal{LP}}}(s)) \\
		&= \sum_{a \in \mathcal{A}}  \sum_{\theta  \in \Theta}  \mu_\theta \Psi^a_{\theta} u^\textnormal{s}_\theta (a^{\phi^{\textnormal{LP}}}(s^a)) \\
		&\ge \sum_{a \in \mathcal{A}}  \sum_{\theta  \in \Theta}  \mu_\theta \Psi^a_{\theta} u^\textnormal{s}_\theta (a) \\
		&\ge \sum_{a \in \mathcal{A}}  \sum_{\theta  \in \Theta}  \widehat{\mu}_\theta \Psi^a_{\theta} u^\textnormal{s}_\theta (a) - \left|\sum_{\theta \in \Theta} \widehat{\mu}_\theta - \mu_\theta \right| \\
		&\ge \sum_{a \in \mathcal{A}}  \sum_{\theta  \in \Theta}  \widehat{\mu}_\theta \psi^a_{\theta} u^\textnormal{s}_\theta (a) - \left|\sum_{\theta \in \Theta} \widehat{\mu}_\theta - \mu_\theta \right| \\
		&\ge \sum_{a \in \mathcal{A}}  \sum_{\theta  \in \Theta}  \mu_\theta \psi^a_{\theta} u^\textnormal{s}_\theta (a) - 2\left|\sum_{\theta \in \Theta} \widehat{\mu}_\theta - \mu_\theta \right|.
	\end{align*}
	We recall that the value of $\psi$ is at least the optimal value of Program~\ref{eq:lp_two_signals} when $\widehat{\mu} = \mu$, and such a value is at last $\text{OPT}-10\epsilon n d$ (see the proof of Lemma~\ref{lem:decomposition_vertexes}), 
	Thus, we have that:
	\begin{align*}
		u (\phi^{\textnormal{LP}}) \ge \sum_{a \in \mathcal{A}}  \sum_{\theta  \in \Theta}  \mu_\theta \psi^a_{\theta} u^\textnormal{s}_\theta (a) - 2\left|\sum_{\theta \in \Theta} \widehat{\mu}_\theta - \mu_\theta \right| \ge \text{OPT}-10\epsilon n d - 2\left|\sum_{\theta \in \Theta} \widehat{\mu}_\theta - \mu_\theta \right|,
	\end{align*}
	concluding the proof.
\end{proof}
