# Supplementary material for: Online Bayesian Persuasion Without a Clue
Source: arXiv:2411.06141 source file (2024-11-09)
Supplement: Supplementary file 3 [file appendix_hyperplane.tex]

%\begin{algorithm}[H]
%	\caption{\texttt{Find-HS}}\label{alg:find_hyperplane}
%	\begin{algorithmic}[1]
%		\Require $x$
%		\State $x ' \gets \texttt{Find-Interior-Point}(\mathcal{U}_{a_i}, \mathcal{U}_{a_j})$
%		\State $a_k \gets \texttt{Action-Oracle}(x')$
%		\If{$a_k = a_i$}
%		\State $x^1 \gets x'$, $x^2 \gets x$
%		\Else
%		\State $x^1 \gets x$ for any $x \in \mathcal{L}_{a_i}$, $x^2 \gets x'$  
%		\EndIf
%		%\State $y \gets 18 B \epsilon m n^2 + 2  n \eta \sqrt{m}$
%		%\State $D_i\gets \{d_q: \widetilde {H}_{i,q}\neq \emptyset\}$
%		% Set  $p^1$ such that $p^1 \in \lreg_{d_i}$, $p^2 \leftarrow p$, $d \gets \bot$
%		\While{$\| x^1 - x^2 \|_2 > \eta $}\label{line:hyperplane_loop}
%		\State $x^\star_\theta \leftarrow (x^1_\theta + x^2_\theta)/2$ for all $\theta \in \Theta$\Comment{\textcolor{gray}{Middle point of the current line segment}}
%		\State $a_k \leftarrow \texttt{Action-Oracle}(x^\star)$
%		\If {$a_k \not \in \mathcal{A}'$} \label{line:add_hp_1}%\Comment{\textcolor{gray}{Add $d$ to to-be-processed meta-actions in \texttt{Try-Cover}}}
%		\State $\mathcal{L}_{a_k} \gets \{ x \}$, $\mathcal{U}_{a_k} \gets \mathcal{X} $, $\mathcal{C} \gets \mathcal{C} \cup \{a_k\}$, $\mathcal{A}' \gets \mathcal{A}' \cup \{a_k\}$ \label{line:add_2}
%		\EndIf
%		%\If {$d_k = \bot$}
%		%\State \Return $\bot$
%		%\EndIf
%		\If{$a_k = a_i$}
%		\State $x^1 \leftarrow x^\star$
%		\Else
%		\State $x^2 \leftarrow x^\star$
%		\EndIf
%		\EndWhile
%		%\State $p'_\omega \leftarrow (p^1_\omega + p^2_\omega)/2$ for all $\omega \in \Omega$\label{line:calc_hp_1}
%		
%		%\If{$d_j = d_i$} \Comment{\textcolor{gray}{The approximate halfspace $\widetilde{H}_{ik}$ is the first one for $\mathcal{L}_{d_i}$}}
%		%\State $\Delta \widetilde{c}_{ik} \gets \sum\limits_{\omega \in \Omega} \left(  \widetilde{F}_{d_{j},\omega} -  \widetilde{F}_{d_{k},\omega} \right) p_{\omega}' $ \label{line:def_delta_cost_1}
%		%\Else \Comment{\textcolor{gray}{The approximate halfspace $\widetilde{H}_{ij}$ has already been computed}}
%		%\State $\Delta \widetilde{c}_{ik} \gets \Delta \widetilde{c}_{ij} + \sum\limits_{\omega \in \Omega} \left(  \widetilde{F}_{d_{j},\omega} -  \widetilde{F}_{d_{k},\omega} \right) p_{\omega}' $ \label{line:def_delta_cost_2}
%		%\EndIf
%		
%		%\State $\widetilde{H} \coloneqq \left\{ p \in \mathbb{R}_{+}^m \mid \sum\limits_{\omega \in \Omega} \left(  \widetilde{F}_{d_{i},\omega} -  \widetilde{F}_{d_{k},\omega} \right) p_{\omega} \ge \Delta \widetilde{c}_{ik}-y  \right\}$\label{line:calc_hp_2}
%		%\State \textbf{return} $(\widetilde{H},d_k)$
%	\end{algorithmic}
%\end{algorithm}
