# Supplementary material for: Online Bayesian Persuasion Without a Clue
Source: arXiv:2411.06141 source file (2024-11-09)
Supplement: Supplementary file 4 [file appendix_proofs.tex]

\section{Omitted Proofs}
